# Supplementary material for: SafeBound: A Practical System for Generating Cardinality Bounds
Source: arXiv:2211.09864 source file (2022-11-17)
Supplement: Supplementary file 1 [file appendix.tex]

\section{Appendix}
\subsection{Proof of Theorem \ref{thm:cdf:upper:bound}}
\label{app:cdf:upper:bound}

We begin by introducing some notation from prior work \cite{DBLP:journals/corr/abs-2201-04166}. First, recall that a degree sequence for a relation $R$ and variable $V$ is a vector $\bm f_{R.V}$ such that $f_{R.V,i}$ is the frequency of the $i$th most frequent value, and $F_{R.V,i}=\sum_{j=1,i}f_{R.V,j}$ is the cumulative degree sequence (CDS). We represent relations $R$ as tensors $M_R$ with one dimension for each variable present in the relation. The value at a particular entry $M_{i_1,\ldots,i_{|\bm V_R|}}$ is equal to the frequency of that tuple, $(i_1,\ldots,i_{|\bm V_R|})$, in the relation $R$. Note that entries can be zero if that tuple does not appear in $R$. Additionally, the discrete derivative and integral of a tensor $M$ on a variable $V$ is defined as,
\begin{defn}
\begin{align}
    (\Delta_V M)_{v_i} &= M_{v_i}-M_{v_i-1}\\
    (\Sigma_V M)_{v_i} &= \sum_{j=1,v_i}M_{j} 
\end{align} 
\end{defn}

A tensor $M$ is \textit{consistent} with a set of degree sequences $\bm f_R$ if the following is true,
\begin{align*}
    (\sum_{V'\neq V}M)_i \leq f_{R.V,i}  &  &\forall\,\, i\in \mathbb{D}_V, V\in \bm V_R
\end{align*}
Briefly, this means that if we contract the tensor down to a single dimension, then the resulting vector is less than the DF $F_{R.V}$ at all points. The set $\mathcal{M}_{\bm f_R}$ is the set of tensors consistent with $\bm f_{R}$.

Lastly, we define the \textit{value tensor}, $E^{\bm F_R}$, and use it to explicitly define the \textit{worst-case tensor}, $C^{\bm F_R}$.
\begin{defn} The {\em value} tensor,
  $\bm E^{\bm F_R}\in \R_+^{[\bm n]}$, is defined by the
  following linear optimization problem:
\begin{align}
\forall \bm m \in [\bm n]: && E_{\bm m}^{\bm F_{R}} \defeq  \mbox{\ Maximize:\ } &  \sum_{\bm s \leq \bm m} M_{\bm s}\label{eq:def:v}\\
  && \mbox{Where:\ } & \bm M \in \calM_{\bm f_R}\nonumber
\end{align}
The {\em worst-case} tensor,
$\bm C^{\bm F_R}\in \R^{[\bm n]}$, is defined as:
  \begin{align}
    && \bm C^{\bm f_R} \defeq & \Delta_{V_1}\cdots \Delta_{V_d} \bm E^{\bm F_{R}} \label{eq:def:c}
  \end{align}
Or, equivalently,
 \begin{align}
    && \Sigma_{V_1}\cdots\Sigma_{V_d} \bm C^{\bm f_R} = \bm E^{\bm F_{R}} \label{eq:def:c}
  \end{align}
\end{defn}
Note that this worst-case tensor is equivalent to the worst-case instance, $W(R)$ of a relation $R$, as depicted in Figure \ref{fig:degree:sequence:bound}.

Getting back to Theorem \ref{thm:cdf:upper:bound} of this work, we start by proving that it holds for star queries before expanding to all Berge-acyclic queries. Consider the following query,
\begin{align*}
    Q_{STAR} &= R(V_1,\ldots, V_d)S_1(V_1)\ldots S_d(V_d)
\end{align*}
If $\bm M$ is the count tensor of the relation $R$ and $\bm a^{(V_i)}$ is the count tensor of $S_i$, in this case a simple non-increasing vector, then we can express the query size as follows,
\begin{align*}
    |Q_{STAR}(D)| &= \bm M\cdot \bm a^{(V_1)} \cdots\bm a^{(V_d)}
\end{align*}

Given this notation, we consider part of Theorem 3.2 from \cite{DBLP:journals/corr/abs-2201-04166}.

\begin{thm}\textbf{[Thm. 3.2 from \cite{DBLP:journals/corr/abs-2201-04166}]} \label{th:main:star} Let $\bm f_R$ be the set of degree sequences as above, and let $\bm V, \bm C$ defined
  by~\eqref{eq:def:v}-\eqref{eq:def:c}. Then:
  \begin{enumerate}
  
  \item \label{item:th:main:star:5} We can define the value tensor as follows,
    \begin{align}
      \forall \bm m \in [\bm n]: &&    E_{\bm m}^{\bm F_R} = & \min\left(F_{R.V_1}(m_1), \ldots, F_{R.V_d}(m_d)\right) \label{eq:v:is:max}
    \end{align}
    
  \item \label{item:th:main:star:4} For any non-increasing vectors
    $\bm a^{(V_p)} \in \R_+^{[n_p]}$, $p=2,d$, the vector
    $\bm C^{\bm f_R} \cdot \bm a^{(V_2)} \cdots \bm a^{(V_d)}$ is in
    $\R^{[n_1]}_+$ and non-increasing.
    
  \item \label{item:th:main:star:2} For all count tensors $\bm M_R$, and all non-increasing vectors   $\bm a^{(X_1)} \in \R_+^{[n_1]}, \ldots, \bm a^{(X_d)} \in   \R_+^{[n_d]}$:
  \begin{align}
    \bm M_R \cdot \bm a^{(V_1)} \cdots \bm a^{(V_d)} \leq & \,\,\bm C^{\bm f_R} \cdot \bm a^{(V_1)} \cdots \bm a^{(V_d)}
  \end{align}
  Directly implying,
  \begin{align}
    |Q_{STAR}(D)| \leq & \,\,|Q_{STAR}(W(s(D)))|
  \end{align}

  \end{enumerate}
\end{thm}

Let $\hat{\bm F}_R$ be an upper bound of $\bm F_R$, i.e. $\hat{\bm F}_{R.V}(i) \geq \bm F_{R.V}(i)\,\,\forall\,\,V\in\bm V_R, i$, and define $\hat{f}_{R.V} = \Delta_V\hat{\bm F}_{R.V}$ and $\hat{\bm f}_R$ as the set of these degree sequences which, as specified in Theorem \ref{thm:cdf:upper:bound}, must be non-increasing. Further, note that item \ref{item:th:main:star:5} and item \ref{item:th:main:star:4} relies only on the properties of the worst-case instance's inherent structure, so it immediately applies to $\bm C^{\hat{\bm F}_R}$.

Based on the above, we can prove the following lemma,
\begin{lmm}  \label{lmm:cdf:star}
For all non-increasing vectors   $\bm a^{(V_1)} \in \R_+^{[n_1]}, \ldots, \bm a^{(V_d)} \in   \R_+^{[n_d]}$:
  \begin{align}
    \bm C^{\bm f_R} \cdot \bm a^{(V_1)} \cdots \bm a^{(V_d)}\leq & \,\,\bm C^{\hat{\bm F}_R} \cdot \bm a^{(V_1)} \cdots \bm a^{(V_d)}
  \end{align}
Directly implying, 
  \begin{align}
    |Q_{STAR}(W(s(D)))| \leq & \,\,|Q_{STAR}(W(\Delta\hat{S}))|
  \end{align}
\end{lmm}
\begin{proof}
Following the original proof of item \ref{item:th:main:star:2}, we begin by simplifying the problem using 1-0 vectors. In particular, let $\bm b^{(m)}\in \mathcal{R}^n$ be the vector with $m$ $1$'s followed by $n-m$ $0$'s. Because the $\bm a^{V_i}$ are non-increasing integral vectors, they can be represented as a sum of 1-0 vectors, so it suffices to consider the case where each of them is a 1-0 vector. In this case, the problem description becomes,
\begin{align*}
    \bm C^{\bm f_R} \cdot \bm b^{(m_1)} \cdots \bm b^{(m_d)} \leq & \,\,\bm C^{\hat{\bm F}_R} \cdot \bm b^{(m_1)} \cdots \bm b^{(m_d)}
\end{align*}
Multiplying against $\bm b^{(m)}$ is the same as summing over the first $m$ indices, so this can be alternatively expressed as,
\begin{align*}
    \Sigma_{m_1}\ldots\Sigma_{m_d} \bm C^{\bm f_R} \leq & \,\,\bm \Sigma_{m_1}\ldots\Sigma_{m_d} C^{\hat{\bm f}_R}
\end{align*}
Considering the definition of the value tensor $E^{\bm f_R}_{\bm m}$, we can rephrase this as follows where $\bm m = (m_1,\ldots,m_d)$,
\begin{align*}
    E^{\bm f_R}_{\bm m} \,\,&\leq \,\, E^{\hat{\bm f}_R}_{\bm m}
\end{align*}
Lastly, we insert the alternative definition of $E^{\bm f_R}$ provided in item \ref{item:th:main:star:5} and the fact that each $\hat{\bm F}_{R.V_i}$ is an upper bound of $\bm F_{R.V_i}$ to prove the lemma,
\begin{align*}
    \min(F_{R.V_1}(m_1),\ldots, F_{R.V_d}(m_d))\,\,&\leq \,\, \min(\hat{F}_{R.V_1}(m_1),\ldots, \hat{F}_{R.V_d}(m_d))
\end{align*}
\end{proof}

To prove that this can be extended to general queries, we rely on more theory from \cite{DBLP:journals/corr/abs-2201-04166}.

\begin{thm} \textbf{Implied by Thm. 4.2 of \cite{DBLP:journals/corr/abs-2201-04166}}
  If the following is true for a set of database instances, $\mathcal{D}$,
  \begin{enumerate}
      \item \label{item:th:main:star:4} For any non-increasing vectors
        $\bm a^{(V_p)} \in \R_+^{[n_p]}$, $p=2,d$, the vector
        $\bm C^{\bm f_R} \cdot \bm a^{(V_2)} \cdots \bm a^{(V_d)}$ is in
        $\R^{[n_1]}_+$ and non-increasing.
    
      \item \label{item:th:main:star:2} For all relations $R\in\mathcal{D}$ with count tensor $\bm M_R$, and all non-increasing vectors $\bm a^{(X_1)} \in \R_+^{[n_1]}, \ldots, \bm a^{(X_d)} \in   \R_+^{[n_d]}$:
      \begin{align}
        \bm M_R \cdot \bm a^{(V_1)} \cdots \bm a^{(V_d)} \leq & \,\,\bm C^{\bm f_R} \cdot \bm a^{(V_1)} \cdots \bm a^{(V_d)}
      \end{align}
  \end{enumerate}
  Then, for any Berge-acyclic query, $Q$,
  \begin{align}
      |Q(D)| \leq |Q(W(s))| \quad \forall D\in\mathcal{D}
  \end{align}
\end{thm}

The first immediately holds for $\bm C^{\hat{F}_R}$ from Theorem \ref{th:main:star} while the latter holds for the set of all database instances, $D$, such that $D\models S$ due to Lemma \ref{lmm:cdf:star}.

\subsection{Proof of Theorem \ref{th:lossless:compression}}
\label{app:lossless:compression}
We begin with a simple lemma.
\begin{lmm}\label{lmm:unique:values}
If a degree sequence $\bm f_{R.V}$ has $n$ unique degree values, then it can be represented by an $n$-segment piece-wise constant function.
\end{lmm}
\begin{proof}
Because degree sequences are monotone, it is guaranteed that all instances of a particular degree value will occur sequentially. This means that we can compress the sequence with a run length encoding where $d_i$ is the $i$th highest degree value and $c_i$ is how many times it occurs. This looks like $(d_1,c_1),\ldots,(d_n,c_n)$. We then define our piece-wise constant function with the $i$th segment having value $d_i$ and range $(\sum_{j=1}^{i-1}c_j, \sum_{j=1}^{i}c_j)$ .
\end{proof}

This proof of the theorem then follows from bounding the number of unique degree values that a relation $R$ with max degree $d$ and  size $N$ can have. Because the degree values are positive integers, it is immediate that there cannot be more than $d$ unique values in the range $[1,d]$.

To demonstrate why the sequence cannot have more than $\sqrt{2N} + 1$ unique values, suppose that this is false. Because degree values are positive integers, the the minimum possible sum over these values would be the summation from $1$ to $\sqrt{2N}+1$. 

\begin{align}
    \sum_i^{\sqrt{2N}+1} i & = (\sqrt{2N}+1)(\sqrt{2N}+2)/2\\
    & > (\sqrt{2N})(\sqrt{2N})/2=N
\end{align}
Because this summation must match the number of rows in the relation, $N$, this is a contradiction. Therefore, the relation cannot have over $\sqrt{2N}$ unique degree values.

Because the number of unique values is less than $\min(d, \sqrt{2N})$, by lemma \ref{lmm:unique:values} we can losslessly represent it in a piece-wise constant function of $\min(d,\sqrt{2N})$ segments.
